# Supplementary material for: Subgraph covers -- An information theoretic approach to motif analysis in networks
Source: arXiv:1406.1414 ancillary file (2014-10-01)
Supplement: Supplementary file 1 [file SupplementalMaterial.pdf]

# Supporting Material

In the following, we describe two heuristics for finding optimal instance sets of a motif.

## 1 The Maximum Independent Set Heuristic for Finding Optimal Instance Sets

The maximum independent set heuristic is based on finding maximum independent vertex sets of various intersection graphs of the instances of m.The motivation behind this heuristic is that the larger the number of uncovered edges an m-subgraph contains, the more efficient it is. Therefore when constructing an optimal instance set for a motif m, we start with m-subgraphs that contain the largest number of uncovered edges. Moreover, because these are the most efficient instances, we would like to include a maximal number of such m-subgraphs to the optimal instance set while making sure that these do not share edges. Finding such a set of m-subgraphs is equivalent to finding a maximum independent vertex set of the intersection graph of the m-subgraphs that contain a maximal number of uncovered edges. Also when the subgraphs in a cover are not allowed to share edges, finding a maximum independent set of m-subgraphs and finding an optimal instance set of m are equivalent. The intersection graph of m-subgraphs containing n covered edges is defined as follows: the vertices of this graph are all the m-subgraphs of G that contain n covered edges and there is an edge between two vertices whenever they have at least one uncovered edge in common. The problem of finding a maximal independent set is known to be NP-hard therefore a heuristic has to be used. Once a maximum independent vertex set is found, subgraphs in this set are stepwise added to the m-set provided they increase the overall efficiency (decreases $\sigma$) of the optimal instance set constructed so far. When all the m-subgraphs with intersection number n are exhausted, the set of covered edges is updated and the procedure is repeated for n+1 until there remains no m-subgraph that decreases $\sigma$.

**Algorithm 1** Maximum-IS heuristic for OptimalInstanceSet(G,m,CoveredEdges)

$mSet = SubGraphInstances(G, m), OIS(m) = \emptyset$
**for** n:=0 until e(m)-1 **do**
  $IG = IntersectionGraph(mSet, CoveredEdges \cup Edges(OIS(m)), n)$
  MIS=MaximumIndependentSet(IG) ▷ Maximum independent set heuristic
  **while** $MIS \neq \emptyset$ **do**
    s=random pick from MIS
    **if** $\sigma(m, OIS(m)) \leq \sigma(m, OIS(m) \cup \{s\})$ **then**
      $OIS(m) \leftarrow OIS(m) \cup \{s\}$
      $MIS \leftarrow MIS - \{s\}$
    **else**
      end while, end for
    **end if**
  **end while**
**end for**
**return** OIS(m)
**function** IntersectionGraph(mSet,CoveredEdges,n)
  $V = \{m \in mSet : |Edges(m) \cap CoveredEdges| = n\}$
  $E = \{\{m, m\prime\} : m, m\prime \in mSet$ and $Edges(m) \cap Edges(m\prime) - CoveredEdges \neq \emptyset\}$
  **return** G(E,V)
**end function**

Here MaximumIndependentSet is a heuristic for finding the maximum independent sets and SubGraphInstances(G,m) [1, 2] is a function that finds and returns all instances of m in G. A large variety of heuristics for finding maximum independent sets of varying computational complexity can be found in the literature [3].

### 1.0.1 Maximal Independent Set Heuristic

Finding the maximum independent set of various intersection graphs at each step of the greedy algorithm sometimes requires a large amount of computational resources since some subgraphs might occur in very large numbers. As a result the corresponding intersection graphs also can become very large. For instance, in some networks that have on the order of 1000 nodes some 5 node graphs appear hundreds of thousand or even million times. Moreover such high frequency subgraphs also intersect quite heavily thus their intersection graph can occupy a lot of memory. To overcome this we introduce a lighter/faster version of the above algorithm which uses maximal independent sets instead of maximum independent sets. Maximal independent vertex sets are independent sets that are not a subset of any other independent set. Finding a maximal independent set is much easier that finding a maximum independent set. One can easily obtain an maximal in dependent set of m-subgraphs by stepwise picking an instance of m, removing the edges of m from the graph and the repeating the procedure until the graph contains no more copies of m. The maximal independent set of subgraphs is then used as a candidate for the optimal instance

set.

**Algorithm 2** Maximal-IS heuristic for OptimalInstance-Set(G,m,CoveredEdges)

$OIS(m) = \emptyset$
remove CoveredEdges from G
**while** $Subgraph(G, m) \neq \emptyset$ **do**
  $s = Subgraph(G, m)$ ▷ Find an m-subgraph of G
  $OIS(m) \leftarrow OIS(m) \cup \{s\}$
  remove edges in $s$ from $G$
**end while**
**return** OIS(m)

Using maximal independent sets instead of maximum independent sets introduces more variability in terms of the cover obtained by the greedy heuristic. The maximal independent set heuristic also always produces non-intersecting subgraphs covers. However, the heuristic can be easily be modified to allow intersections between subgraphs in the cover. This essentially would correspond to approximating the maximum independent sets by maximal ones in the first algorithm. However in applications, including such intersecting subgraphs did not result in covers with significantly lower total information. On the other hand this heuristic does not require all subgraphs and their intersection graphs to be computed and stored in memory which makes it much more suitable for larger networks and motifs when computational resources are limited.

## 1.1 Discussion

Due to its probabilistic nature, the greedy heuristic might find different covers for the same networks on different runs. When using the greedy heuristic, this variability essentially comes from the heuristic used to obtain optimal instance sets. More specifically in the case of the maximum independent set heuristic the source of this variability is the heuristic used to approximate maximum independent sets. In general one expects that heuristics which are able to find better solutions (that is larger independent sets) to also have less variability. The maximal independent set heuristic can be seen as the crudest way to approximate maximum independent sets and as a result one also expects it to have the largest variability. In general the variability of the optimal instance sets obtained by the different heuristics also strongly depends on the network. Depending on whether the greedy algorithm is able to produce a stable solution or not, one can opt for more sophisticated algorithms to approximate maximum independent sets. However, as exemplified by the maximum and maximal independent set heuristics, this in general might involve significant trade offs in terms of computational complexity. On the other hand, one can also devise heuristics that do not rely on independent sets for finding optimal instance sets.

However, for the networks we considered, we observed that the results of greedy heuristics are quite stable over runs even when the maximal independent set heuristic is used. Although for some networks the motif sets obtained on different runs differ, these are mostly restricted to motifs that only occur a few times in the cover or are one node intersections of smaller motifs. For instance,

one cover might contain triangles and the other subgraphs that are made of two triangles connected at one node.

# References

[1] Luigi P Cordella, Pasquale Foggia, Carlo Sansone, and Mario Vento. A (sub) graph isomorphism algorithm for matching large graphs. *Pattern Analysis and Machine Intelligence, IEEE Transactions on*, 26(10):1367–1372, 2004.

[2] Julian R Ullmann. An algorithm for subgraph isomorphism. *Journal of the ACM (JACM)*, 23(1):31–42, 1976.

[3] Magnús M Halldórsson. Approximations of independent sets in graphs. In *Approximation algorithms for combinatiorial optimization*, pages 1–13. Springer, 1998.
